# Supplementary material for: Second Order Methods for Bandit Optimization and Control
Source: arXiv:2402.08929 source file (2024-10-03)
Supplement: Supplementary file 1 [file appendix-proper.tex]

\section{Regret of Bandit Newton Method for Proper Learning (Section~\ref{sec:proper-learning})}
% \subsection{Intermediate Results}
% We first present some useful intermediate results. 
% \begin{lemma}
%     \label{lem:bandit-newton-proper-proof}
%     Algorithm~\ref{alg:simple-bqo-proper} is a proper learning algorithm. That is, the iterates $\{y_t\}_{t=1}^T$ generated by the algorithm belong to the constraint set $\K$
% \end{lemma}
% \begin{proof}
%     The proof relies on Dikin Ellipsoid property of SCBs. Observe that $\|y_t-x_t\|_{\tilde{A}_{t}} = \frac{1}{2} \tilde{A}_{t}^{-\frac{1}{2}}(v_{t,1}+v_{t,2})$
% \end{proof}
\subsection{Properties of Iterates}
\begin{lemma}
\label{lem:concentration-cumulative-hessian-proper} 
Define the smoothed function $\smoothfBB{t}$ as
$$
\smoothfBB{t}(x) \coloneqq \E_{u\sim \ball, v \sim \ball}\left[f_t\left(x + \frac{1}{4} \tilde{A}_{t}^{-\frac{1}{2}}(u+v)\right)\right].
$$
Let $\tilde{A}_t=\nabla^2R(x_t)+\frac{\eta}{\kappa'}\sum_{s=0}^{t-1}\tilde{H}_{s}$, and $A_t=\nabla^2R(x_t)+\frac{\eta}{\kappa'}\sum_{s=0}^{t-1}\nabla^2\smoothfBB{s}(x_s)$. 
%Let $B^*=B+\sqrt{2}(G+\sqrt{2}C)$. 
Suppose $\eta\le \kappa'(12d^2B\sqrt{T})\log(dT^2))^{-1}$. Then, $\forall t$, with probability at least $1-\frac{t}{T^2}$, the following properties holds for every $s\le t$,
\begin{enumerate}
    \item $\tilde{A}_s$ is close to $A_s$
    \begin{align*}
\|I-A_{s}^{-\frac{1}{2}}\tilde{A}_sA_{s}^{-\frac{1}{2}}\|_2\le \frac{1}{2}.
\end{align*}
     \item $y_s$ lies in the constraint set $\K$
\end{enumerate}
\end{lemma}
\begin{proof}
\noindent We prove the result using induction.

\paragraph{Base case ($t=1$).} Since $\tilde{A}_1 = A_1 = \nabla^2R(x_1)$, the first part holds trivially. Using Dikin Ellipsoid property of SCBs, we can also conclude that $y_1 \in \K$.
\paragraph{Induction Step.} Suppose the hypothesis holds with probability at least $1-\frac{t-1}{T^2}$ for any $0\le s\le t-1$. We show that the properties hold at iteration $t$. 
% Let $$\tilde{B}_t = I + \frac{\eta}{\kappa'}\sum_{s=0}^{t-1}\tilde{H}_{s}, \quad B_t = I + \frac{\eta}{\kappa'}\sum_{s=0}^{t-1}\nabla^2\smoothfBB{s}(x_s).$$ Since $R(x)$ is $1$-strongly convex, the following holds for any $x\in \K$: $I \preceq B_t \preceq A_t(x)$.
% Now consider the following for any $s\le t$
% \begin{align*}
%     \sup_{x\in \K}\|I-A_{s}(x)^{-\frac{1}{2}}\tilde{A}_s(x)A_{s}(x)^{-\frac{1}{2}}\|_2 &= \sup_{x\in \K}\|A_{s}(x)^{-\frac{1}{2}}(A_s(x)-\tilde{A}_s(x))A_{s}(x)^{-\frac{1}{2}}\|_2\\
%     & = \sup_{x\in \K}\|A_{s}(x)^{-\frac{1}{2}}(B_s-\tilde{B}_s)A_{s}(x)^{-\frac{1}{2}}\|_2\\
%     & \leq \sup_{x\in \K}\|A_{s}(x)^{-\frac{1}{2}}B_s^{1/2}\|_2^2\|B_s^{-1/2}(B_s-\tilde{B}_s)B_s^{-1/2}\|_2\\
%     & \stackrel{(a)}{\leq} \|B_s^{-1/2}(B_s-\tilde{B}_s)B_s^{-1/2}\|_2,
% \end{align*}
% where $(a)$ follows from the previous observation that $B_t \preceq A_t(x)$. The rest of the proof uses similar arguments as in the proof of Lemma~\ref{lem:concentration-cumulative-hessian}, where we showed that $\|B_s^{-1/2}(B_s-\tilde{B}_s)B_s^{-1/2}\|_2 \leq \frac{1}{2}$ holds with high probability.
Consider the following
\begin{align*}
A_t^{-1/2}(A_t-\tilde{A}_t)A_t^{-1/2}&=\frac{\eta}{\kappa'} \sum_{s=1}^t A_{t}^{-\frac{1}{2}}(\E[\tilde{H}_s\mid \F_{s-1}]-\tilde{H}_s)A_{t}^{-\frac{1}{2}},
\end{align*}
where $Z_s=A_{t}^{-\frac{1}{2}}(\E[\tilde{H}_s\mid \F_{s-1}]-\tilde{H}_s)A_{t}^{-\frac{1}{2}}$ forms a martingale sequence with respect to the filtration $\F_{s}$. Here, we used the fact that $\E[\tilde{H}_s\mid \F_{s-1}] = \nabla^2\smoothfBB{s}(x_s).$ Furthermore, note that by definition of $\tilde{H}_s$, since $-2I\preceq v_{t,1}v_{t,2}^{\top}+v_{t,2}v_{t,1}^{\top}\preceq 2I$, we have
\begin{align*}
\forall s \le t-1, \quad -16d^2B\tilde{A}_{s}\preceq \tilde{H}_s\preceq 16d^2B\tilde{A}_{s}.
\end{align*}
Thus, with probability at least $1-\frac{t-1}{T^2}$, $\forall s\le t-1$,
\begin{align*}
Z_s\preceq A_{t}^{-\frac{1}{2}}\left(32d^2B\tilde{A}_{s}\right)A_{t}^{-\frac{1}{2}}\preceq \textcolor{red}{32d^2B A_{s}^{-\frac{1}{2}}\tilde{A}_{s}A_{s}^{-\frac{1}{2}}},
\end{align*}
and 
\begin{align*}
Z_s\succeq A_t^{-\frac{1}{2}} \left(-16d^2B^*\tilde{A}_{s-1}\right) A_t^{-\frac{1}{2}}\succeq \textcolor{red}{-16d^2B^* A_{s-1}^{-\frac{1}{2}}\tilde{A}_{s-1}A_{s-1}^{-\frac{1}{2}}}.
\end{align*}
\textcolor{red}{We need some relation between $A_s$ and $A_t$ that can help us bound $A_t^{-1/2}A_s^{1/2}$}.

\js{Is it possible if we take $A_t=\max_{t\in[T]}\nabla^2 R(x_t)+\sum_{s=0}^{t-1}\nabla^2 \tilde{f}_{s}^{\ball,\ball}(x_s)$?}

\end{proof}

\subsection{Proof of Theorem~\ref{thm:expected_regret_bound}}
Similar to the proof of Theorem~\ref{thm:expected_regret_bound}, we first define the following smoothed functions 
\begin{align*}
&\smoothfBB{t}(x) \coloneqq \E_{u\sim \ball, v \sim \ball}\left[f_t\left(x + \frac{1}{2} \tilde{A}_{t-1}^{-\frac{1}{2}}(u+v)\right)\right]\\
&\smoothfBS{t}(x) \coloneqq \E_{u\sim \ball, v \sim \sphere}\left[f_t\left(x + \frac{1}{2} \tilde{A}_{t-1}^{-\frac{1}{2}}(u+v)\right)\right]\\
&\smoothfSS{t}(x) \coloneqq \E_{u\sim \sphere, v \sim \sphere}\left[f_t\left(x + \frac{1}{2} \tilde{A}_{t-1}^{-\frac{1}{2}}(u+v)\right)\right].
\end{align*}
Observe that
\begin{align*}
\E[f_t(y_t)\mid \F_{t-1}]=\smoothfSS{t}(x_t),
\end{align*}
where $\F_t$ denotes the filtration generated by $\{v_{s,1},v_{s,2}\}_{s=1}^{t}$. 
% \eh{here is how I think this proof should be idealy structured:
% \begin{enumerate}
%     \item have a generic theorem about the regret of online newton method with approximate hessian and gradient, that includes a bias term
%     \item proof that the estimators have bias bounded by such and such
%     \item now conclude the regret bound
% \end{enumerate} 
% see the proof for FKM in my book for such a proof but using only gradient. 
% }
By Stokes' theorem~\citep{flaxman2004online}, we have that the gradient and Hessian estimators constructed in Algorithm~\ref{alg:simple-bqo} satisfy 
\begin{align*}
    &\E[\tilde{\nabla}_t\mid \F_{t-1}] = \nabla \smoothfBS{t}(x_t),\quad \E[\tilde{H}_t\mid \F_{t-1}] = \nabla^2 \smoothfBB{t}(x_t).
\end{align*}
Throughout the proof we assume that the cumulative Hessian concentrates well around the true cumulative Hessian:
\begin{align*}
\forall s\in [T], \ \|I-A_{s}^{-\frac{1}{2}}\tilde{A}_sA_{s}^{-\frac{1}{2}}\|_2\le \frac{1}{2}.
\end{align*}

\begin{lemma}[Stability]
\label{lem:bco_scb_stability}
Let $A_t = \left(\nabla^2 R(x_t) + \sum_{s=0}^{t-1}\eta/\kappa' \nabla^2\smoothfBB{s}(x_s)\right).$ 
For any $t \leq T$
\begin{align*}
\|x_{t+1}-x_t\|_{A_{t}} = O(\eta\|\nabla \smoothfBS{t}(x_t)\|_{A_t}^*).    
\end{align*}
\end{lemma}
\begin{proof}
Recall, $x_{t+1}$ is the minimizer of the following objective
\[
x_{t+1} = \argmin_{x\in \K} \eta\left\langle\tilde{\nabla}_t, x\right\rangle + \bregt{t+1}(x,x_{t})
\]
From the first order optimality conditions, we have
\begin{align}
\label{eqn:xt_opt_condition}
    \forall x \in \K, \quad \iprod{\nabla R_{t+1}(x_{t+1}) -\nabla R_{t+1}(x_{t})  + \eta\nabla \smoothfBS{t}(x_t)}{x-x_{t+1}} \geq 0.
\end{align}
Replacing $x$ in the above equation with $x_t$ and rearranging terms gives us
\begin{align*}
   \iprod{\nabla R(x_{t+1}) -\nabla R(x_{t}) +  \eta\nabla \smoothfBS{t}(x_t) + \sum_{s=1}^{t}\frac{\eta}{\kappa'} H_s(x_{t+1}-x_{t})}{x_{t+1}-x_{t}} \leq 0.
\end{align*}
Now suppose $\|x_{t+1}-x_{t}\|_{A_{t}} > \eta\|\nabla \smoothfBB{t}(x_t)\|_{A_t}^*$. Then we have
\begin{align*}
    &\iprod{\nabla R(x_{t+1}) -\nabla R(x_t)  + \eta \nabla f_t(x_t) + \sum_{s=1}^t\eta H_s(x_{t+1}-x_t)}{x_{t+1}-x_t} \\
    &\quad \stackrel{(a)}{\geq}  \frac{\|x_{t+1}-x_t\|_{\nabla^2R(x_t)}^2}{1+\|x_{t+1}-x_t\|_{\nabla^2R(x_t)}} + \eta\|x_{t+1}-x_t\|_{H_{1:t}}^2 +  \iprod{\eta \nabla f_t(x_t)}{x_{t+1}-x_t}\\
    &\quad \stackrel{(b)}{\geq} \frac{\|x_{t+1}-x_t\|_{\nabla^2R(x_t)}^2}{1+\|x_{t+1}-x_t\|_{\nabla^2R(x_t)}}  + \eta\|x_{t+1}-x_t\|_{H_{1:t}}^2- \eta \|\nabla f_t(x_t)\|^*_{A_t}\|x_{t+1}-x_t\|_{A_t},
\end{align*}
where $(a)$ follows from property P3 of SCBs stated in Appendix~\ref{sec:scb} and $(b)$ follows from the fact that $H_t$ is a positive semi-definite matrix. Here $H_{1:t} = \sum_{s=1}^t H_{s}$. Continuing
\begin{align*}
    &\iprod{\nabla R(x_{t+1}) -\nabla R(x_t)  + \eta \nabla f_t(x_t) + \sum_{s=1}^t\eta H_s(x_{t+1}-x_t)}{x_{t+1}-x_t} \\
    &\quad \stackrel{(b)}{\geq} \frac{\|x_{t+1}-x_t\|_{A_t}^2}{1+\|x_{t+1}-x_t\|_{A_t}}  - \eta \|\nabla f_t(x_t)\|^*_{A_t}\|x_{t+1}-x_t\|_{A_t},
\end{align*}
Next, consider the following
% \begin{align*}
%     (\| \gest{t}\|_{M_t}^*)^2 &= \gest{t}^TM_t^{-1}\gest{t} = \lambda^{-2}d^2 f_t^2(\y_t) \v_{1,t}^T\v_{1,t} \leq \lambda^{-2}d^2 B^2.
% \end{align*}
Substituting this in the previous inequality and using the fact that $\|x_{t+1}-x_t\|_{A_t} > 2\lambda^{-1}dB\eta_t$ gives us
\begin{align*}
&\iprod{\nabla R(\x_{t+1}) -\nabla R(\x_t)  + \eta_t \gest{t} + \sum_{s=1}^t\eta_s \hest{s}(\x_{t+1}-\x_t)}{\x_{t+1}-\x_t} \\
&\quad \geq \lambda^{-1}dB\eta_t\|\x_{t+1}-\x_t\|_{M_t} \left(\frac{2}{1+2\lambda^{-1}dB\eta_t} -  1 \right)\\
&\quad \stackrel{(a)}{>} 0,
\end{align*}
where $(a)$ follows from the fact that $\lambda^{-1}dB\eta_t < 1/2.$  This contradicts the first order optimality condition in Equation~\eqref{eqn:}.
This shows that $\|\x_{t+1}-\x_t\|_{M_t} \leq 2\lambda^{-1}dB\eta_t.$ 
\end{proof}

\begin{lemma}
\label{lem:btl}
For any $t \leq T,$ and any $x\in \K$
$$\iprod{\tilde{\nabla}_{t}}{x_{t+1}-x} \leq \frac{\|x-x_t\|^2_{A_t} - \|x-x_{t+1}\|^2_{A_t}}{2\eta}$$.
\end{lemma}
\begin{proof}
    Observe that $x_{t+1}$ can be rewritten as
    \[
    x_{t+1} = \argmin_{x\in \K} \|x-(x_t-\eta A_t^{-1}\tilde{\nabla}_{t})\|_{A_t}^2.
    \]
    From first order optimality conditions, we have the following for any $x\in \K$
    \begin{align*}
        \iprod{x_{t+1} - x_t + \eta A_t^{-1}\tilde{\nabla}_{t}}{x-x_{t+1}}_{A_t} \geq 0
    \end{align*}
    Rearranging terms in the above inequality gives us the required result.
\end{proof}
